# Supplementary material for: Implicit Pairs for Boosting Unpaired Image-to-Image Translation
Source: arXiv:1904.06913 source file (2020-12-03)
Supplement: Supplementary file 1 [file supplamentary.tex]

\input{supplamentary/text.tex}

\input{supplamentary/cityscapes_results.tex}

% \section{Pseudo-pairs results}

\input{supplamentary/baseline_results.tex}

\input{supplamentary/ratio_results.tex}

\input{supplamentary/settings_results.tex}
