# Supplementary material for: Implicit Pairs for Boosting Unpaired Image-to-Image Translation
Source: arXiv:1904.06913 source file (2020-12-03)
Supplement: Supplementary file 2 [file smiling_qualitative_old.tex]

% \begin{figure}
%   \centering% 
 


% \jsubfig{\includegraphics[height=1.6cm]{latex/images/supplamentary/ratio_results/smiling_parameters_pairing_ratio_experiment/001411_real_A_smiling_paired_2000_2000_a2.png}} 
%  {}% 
% \hspace{3pt}
% \hfill%
% \jsubfig{\includegraphics[height=1.6cm]{latex/images/supplamentary/ratio_results/smiling_parameters_pairing_ratio_experiment/001411_fake_B_smiling_2000_with_2000_ratio_05_merged_eyeglasses4000_results.png}} 
%  {}% 
% \hfill%
% \jsubfig{\includegraphics[height=1.6cm]{latex/images/supplamentary/ratio_results/smiling_parameters_pairing_ratio_experiment/001411_fake_B_smiling_paired_2000_2000_a2_merged_eyeglasses4000_results.png}} 
%  {}% 
% \hfill%
% \jsubfig{\includegraphics[height=1.6cm]{latex/images/supplamentary/ratio_results/smiling_parameters_pairing_ratio_experiment/001411_fake_B_smiling_2000_with_2000_asize_200_merged_eyeglasses4000_results.png}} 
%  {}% 
% \hfill%
% \jsubfig{\includegraphics[height=1.6cm]{latex/images/supplamentary/ratio_results/smiling_parameters_pairing_ratio_experiment/001411_fake_B_smiling_2000_with_2000_asize_0_merged_eyeglasses4000_results.png}} 
%  {}% 
% \hfill%
% \\  



% % \jsubfig{\includegraphics[height=1.6cm]{latex/images/supplamentary/ratio_results/smiling_parameters_pairing_ratio_experiment/001424_real_A_smiling_paired_2000_2000_a2.png}} 
% %  {}% 
% % \hspace{3pt}
% % \hfill%
% % \jsubfig{\includegraphics[height=1.6cm]{latex/images/supplamentary/ratio_results/smiling_parameters_pairing_ratio_experiment/001424_fake_B_smiling_2000_with_2000_ratio_05_merged_eyeglasses4000_results.png}} 
% %  {}% 
% % \hfill%
% % \jsubfig{\includegraphics[height=1.6cm]{latex/images/supplamentary/ratio_results/smiling_parameters_pairing_ratio_experiment/001424_fake_B_smiling_paired_2000_2000_a2_merged_eyeglasses4000_results.png}} 
% %  {}% 
% % \hfill%
% % \jsubfig{\includegraphics[height=1.6cm]{latex/images/supplamentary/ratio_results/smiling_parameters_pairing_ratio_experiment/001424_fake_B_smiling_2000_with_2000_asize_200_merged_eyeglasses4000_results.png}} 
% %  {}% 
% % \hfill%
% % \jsubfig{\includegraphics[height=1.6cm]{latex/images/supplamentary/ratio_results/smiling_parameters_pairing_ratio_experiment/001424_fake_B_smiling_2000_with_2000_asize_0_merged_eyeglasses4000_results.png}} 
% %  {}% 
% % \hfill%
% % \\  



% \jsubfig{\includegraphics[height=1.6cm]{latex/images/supplamentary/ratio_results/smiling_parameters_pairing_ratio_experiment/001504_real_A_smiling_paired_2000_2000_a2.png}} 
%  {}% 
% \hspace{3pt}
% \hfill%
% \jsubfig{\includegraphics[height=1.6cm]{latex/images/supplamentary/ratio_results/smiling_parameters_pairing_ratio_experiment/001504_fake_B_smiling_2000_with_2000_ratio_05_merged_eyeglasses4000_results.png}} 
%  {}% 
% \hfill%
% \jsubfig{\includegraphics[height=1.6cm]{latex/images/supplamentary/ratio_results/smiling_parameters_pairing_ratio_experiment/001504_fake_B_smiling_paired_2000_2000_a2_merged_eyeglasses4000_results.png}} 
%  {}% 
% \hfill%
% \jsubfig{\includegraphics[height=1.6cm]{latex/images/supplamentary/ratio_results/smiling_parameters_pairing_ratio_experiment/001504_fake_B_smiling_2000_with_2000_asize_200_merged_eyeglasses4000_results.png}} 
%  {}% 
% \hfill%
% \jsubfig{\includegraphics[height=1.6cm]{latex/images/supplamentary/ratio_results/smiling_parameters_pairing_ratio_experiment/001504_fake_B_smiling_2000_with_2000_asize_0_merged_eyeglasses4000_results.png}} 
%  {}% 
% \hfill%
% \\  



% \jsubfig{\includegraphics[height=1.6cm]{latex/images/supplamentary/ratio_results/smiling_parameters_pairing_ratio_experiment/001516_real_A_smiling_paired_2000_2000_a2.png}} 
%  {}% 
% \hspace{3pt}
% \hfill%
% \jsubfig{\includegraphics[height=1.6cm]{latex/images/supplamentary/ratio_results/smiling_parameters_pairing_ratio_experiment/001516_fake_B_smiling_2000_with_2000_ratio_05_merged_eyeglasses4000_results.png}} 
%  {}% 
% \hfill%
% \jsubfig{\includegraphics[height=1.6cm]{latex/images/supplamentary/ratio_results/smiling_parameters_pairing_ratio_experiment/001516_fake_B_smiling_paired_2000_2000_a2_merged_eyeglasses4000_results.png}} 
%  {}% 
% \hfill%
% \jsubfig{\includegraphics[height=1.6cm]{latex/images/supplamentary/ratio_results/smiling_parameters_pairing_ratio_experiment/001516_fake_B_smiling_2000_with_2000_asize_200_merged_eyeglasses4000_results.png}} 
%  {}% 
% \hfill%
% \jsubfig{\includegraphics[height=1.6cm]{latex/images/supplamentary/ratio_results/smiling_parameters_pairing_ratio_experiment/001516_fake_B_smiling_2000_with_2000_asize_0_merged_eyeglasses4000_results.png}} 
%  {}% 
% \hfill%
% \\  



% \jsubfig{\includegraphics[height=1.6cm]{latex/images/supplamentary/ratio_results/smiling_parameters_pairing_ratio_experiment/001536_real_A_smiling_paired_2000_2000_a2.png}} 
%  {}% 
% \hspace{3pt}
% \hfill%
% \jsubfig{\includegraphics[height=1.6cm]{latex/images/supplamentary/ratio_results/smiling_parameters_pairing_ratio_experiment/001536_fake_B_smiling_2000_with_2000_ratio_05_merged_eyeglasses4000_results.png}} 
%  {}% 
% \hfill%
% \jsubfig{\includegraphics[height=1.6cm]{latex/images/supplamentary/ratio_results/smiling_parameters_pairing_ratio_experiment/001536_fake_B_smiling_paired_2000_2000_a2_merged_eyeglasses4000_results.png}} 
%  {}% 
% \hfill%
% \jsubfig{\includegraphics[height=1.6cm]{latex/images/supplamentary/ratio_results/smiling_parameters_pairing_ratio_experiment/001536_fake_B_smiling_2000_with_2000_asize_200_merged_eyeglasses4000_results.png}} 
%  {}% 
% \hfill%
% \jsubfig{\includegraphics[height=1.6cm]{latex/images/supplamentary/ratio_results/smiling_parameters_pairing_ratio_experiment/001536_fake_B_smiling_2000_with_2000_asize_0_merged_eyeglasses4000_results.png}} 
%  {}% 
% \hfill%
% \\  



% % \jsubfig{\includegraphics[height=1.6cm]{latex/images/supplamentary/ratio_results/smiling_parameters_pairing_ratio_experiment/003523_real_A_smiling_paired_2000_2000_a2.png}} 
% %  {}% 
% % \hspace{3pt}
% % \hfill%
% % \jsubfig{\includegraphics[height=1.6cm]{latex/images/supplamentary/ratio_results/smiling_parameters_pairing_ratio_experiment/003523_fake_B_smiling_2000_with_2000_ratio_05_merged_eyeglasses4000_results.png}} 
% %  {}% 
% % \hfill%
% % \jsubfig{\includegraphics[height=1.6cm]{latex/images/supplamentary/ratio_results/smiling_parameters_pairing_ratio_experiment/003523_fake_B_smiling_paired_2000_2000_a2_merged_eyeglasses4000_results.png}} 
% %  {}% 
% % \hfill%
% % \jsubfig{\includegraphics[height=1.6cm]{latex/images/supplamentary/ratio_results/smiling_parameters_pairing_ratio_experiment/003523_fake_B_smiling_2000_with_2000_asize_200_merged_eyeglasses4000_results.png}} 
% %  {}% 
% % \hfill%
% % \jsubfig{\includegraphics[height=1.6cm]{latex/images/supplamentary/ratio_results/smiling_parameters_pairing_ratio_experiment/003523_fake_B_smiling_2000_with_2000_asize_0_merged_eyeglasses4000_results.png}} 
% %  {}% 
% % \hfill%
% % \\  

% % \jsubfig{\includegraphics[height=1.6cm]{latex/images/supplamentary/ratio_results/smiling_parameters_pairing_ratio_experiment/003529_real_A_smiling_paired_2000_2000_a2.png}} 
% %  {}% 
% % \hspace{3pt}
% % \hfill%
% % \jsubfig{\includegraphics[height=1.6cm]{latex/images/supplamentary/ratio_results/smiling_parameters_pairing_ratio_experiment/003529_fake_B_smiling_2000_with_2000_ratio_05_merged_eyeglasses4000_results.png}} 
% %  {}% 
% % \hfill%
% % \jsubfig{\includegraphics[height=1.6cm]{latex/images/supplamentary/ratio_results/smiling_parameters_pairing_ratio_experiment/003529_fake_B_smiling_paired_2000_2000_a2_merged_eyeglasses4000_results.png}} 
% %  {}% 
% % \hfill%
% % \jsubfig{\includegraphics[height=1.6cm]{latex/images/supplamentary/ratio_results/smiling_parameters_pairing_ratio_experiment/003529_fake_B_smiling_2000_with_2000_asize_200_merged_eyeglasses4000_results.png}} 
% %  {}% 
% % \hfill%
% % \jsubfig{\includegraphics[height=1.6cm]{latex/images/supplamentary/ratio_results/smiling_parameters_pairing_ratio_experiment/003529_fake_B_smiling_2000_with_2000_asize_0_merged_eyeglasses4000_results.png}} 
% %  {}% 
% % \hfill%
% % \\  



% \jsubfig{\includegraphics[height=1.6cm]{latex/images/supplamentary/ratio_results/smiling_parameters_pairing_ratio_experiment/003584_real_A_smiling_paired_2000_2000_a2.png}} 
%  {}% 
% \hspace{3pt}
% \hfill%
% \jsubfig{\includegraphics[height=1.6cm]{latex/images/supplamentary/ratio_results/smiling_parameters_pairing_ratio_experiment/003584_fake_B_smiling_2000_with_2000_ratio_05_merged_eyeglasses4000_results.png}} 
%  {}% 
% \hfill%
% \jsubfig{\includegraphics[height=1.6cm]{latex/images/supplamentary/ratio_results/smiling_parameters_pairing_ratio_experiment/003584_fake_B_smiling_paired_2000_2000_a2_merged_eyeglasses4000_results.png}} 
%  {}% 
% \hfill%
% \jsubfig{\includegraphics[height=1.6cm]{latex/images/supplamentary/ratio_results/smiling_parameters_pairing_ratio_experiment/003584_fake_B_smiling_2000_with_2000_asize_200_merged_eyeglasses4000_results.png}} 
%  {}% 
% \hfill%
% \jsubfig{\includegraphics[height=1.6cm]{latex/images/supplamentary/ratio_results/smiling_parameters_pairing_ratio_experiment/003584_fake_B_smiling_2000_with_2000_asize_0_merged_eyeglasses4000_results.png}} 
%  {}% 
% \hfill%
% \\  



% \jsubfig{\includegraphics[height=1.6cm]{latex/images/supplamentary/ratio_results/smiling_parameters_pairing_ratio_experiment/003588_real_A_smiling_paired_2000_2000_a2.png}} 
%  {}% 
% \hspace{3pt}
% \hfill%
% \jsubfig{\includegraphics[height=1.6cm]{latex/images/supplamentary/ratio_results/smiling_parameters_pairing_ratio_experiment/003588_fake_B_smiling_2000_with_2000_ratio_05_merged_eyeglasses4000_results.png}} 
%  {}% 
% \hfill%
% \jsubfig{\includegraphics[height=1.6cm]{latex/images/supplamentary/ratio_results/smiling_parameters_pairing_ratio_experiment/003588_fake_B_smiling_paired_2000_2000_a2_merged_eyeglasses4000_results.png}} 
%  {}% 
% \hfill%
% \jsubfig{\includegraphics[height=1.6cm]{latex/images/supplamentary/ratio_results/smiling_parameters_pairing_ratio_experiment/003588_fake_B_smiling_2000_with_2000_asize_200_merged_eyeglasses4000_results.png}} 
%  {}% 
% \hfill%
% \jsubfig{\includegraphics[height=1.6cm]{latex/images/supplamentary/ratio_results/smiling_parameters_pairing_ratio_experiment/003588_fake_B_smiling_2000_with_2000_asize_0_merged_eyeglasses4000_results.png}} 
%  {}% 
% \hfill%
% \\  



% \jsubfig{\includegraphics[height=1.6cm]{latex/images/supplamentary/ratio_results/smiling_parameters_pairing_ratio_experiment/003615_real_A_smiling_paired_2000_2000_a2.png}} 
%  {}% 
% \hspace{3pt}
% \hfill%
% \jsubfig{\includegraphics[height=1.6cm]{latex/images/supplamentary/ratio_results/smiling_parameters_pairing_ratio_experiment/003615_fake_B_smiling_2000_with_2000_ratio_05_merged_eyeglasses4000_results.png}} 
%  {}% 
% \hfill%
% \jsubfig{\includegraphics[height=1.6cm]{latex/images/supplamentary/ratio_results/smiling_parameters_pairing_ratio_experiment/003615_fake_B_smiling_paired_2000_2000_a2_merged_eyeglasses4000_results.png}} 
%  {}% 
% \hfill%
% \jsubfig{\includegraphics[height=1.6cm]{latex/images/supplamentary/ratio_results/smiling_parameters_pairing_ratio_experiment/003615_fake_B_smiling_2000_with_2000_asize_200_merged_eyeglasses4000_results.png}} 
%  {}% 
% \hfill%
% \jsubfig{\includegraphics[height=1.6cm]{latex/images/supplamentary/ratio_results/smiling_parameters_pairing_ratio_experiment/003615_fake_B_smiling_2000_with_2000_asize_0_merged_eyeglasses4000_results.png}} 
%  {}% 
% \hfill%
% \\  



% \jsubfig{\includegraphics[height=1.6cm]{latex/images/supplamentary/ratio_results/smiling_parameters_pairing_ratio_experiment/002654_real_A_smiling_paired_2000_2000_a2.png}} 
%  {}% 
% \hspace{3pt}
% \hfill%
% \jsubfig{\includegraphics[height=1.6cm]{latex/images/supplamentary/ratio_results/smiling_parameters_pairing_ratio_experiment/002654_fake_B_smiling_2000_with_2000_ratio_05_merged_eyeglasses4000_results.png}} 
%  {}% 
% \hfill%
% \jsubfig{\includegraphics[height=1.6cm]{latex/images/supplamentary/ratio_results/smiling_parameters_pairing_ratio_experiment/002654_fake_B_smiling_paired_2000_2000_a2_merged_eyeglasses4000_results.png}} 
%  {}% 
% \hfill%
% \jsubfig{\includegraphics[height=1.6cm]{latex/images/supplamentary/ratio_results/smiling_parameters_pairing_ratio_experiment/002654_fake_B_smiling_2000_with_2000_asize_200_merged_eyeglasses4000_results.png}} 
%  {}% 
% \hfill%
% \jsubfig{\includegraphics[height=1.6cm]{latex/images/supplamentary/ratio_results/smiling_parameters_pairing_ratio_experiment/002654_fake_B_smiling_2000_with_2000_asize_0_merged_eyeglasses4000_results.png}} 
%  {}% 
% \hfill%
% \\  



% \jsubfig{\includegraphics[height=1.6cm]{latex/images/supplamentary/ratio_results/smiling_parameters_pairing_ratio_experiment/002655_real_A_smiling_paired_2000_2000_a2.png}} 
%  {}% 
% \hspace{3pt}
% \hfill%
% \jsubfig{\includegraphics[height=1.6cm]{latex/images/supplamentary/ratio_results/smiling_parameters_pairing_ratio_experiment/002655_fake_B_smiling_2000_with_2000_ratio_05_merged_eyeglasses4000_results.png}} 
%  {}% 
% \hfill%
% \jsubfig{\includegraphics[height=1.6cm]{latex/images/supplamentary/ratio_results/smiling_parameters_pairing_ratio_experiment/002655_fake_B_smiling_paired_2000_2000_a2_merged_eyeglasses4000_results.png}} 
%  {}% 
% \hfill%
% \jsubfig{\includegraphics[height=1.6cm]{latex/images/supplamentary/ratio_results/smiling_parameters_pairing_ratio_experiment/002655_fake_B_smiling_2000_with_2000_asize_200_merged_eyeglasses4000_results.png}} 
%  {}% 
% \hfill%
% \jsubfig{\includegraphics[height=1.6cm]{latex/images/supplamentary/ratio_results/smiling_parameters_pairing_ratio_experiment/002655_fake_B_smiling_2000_with_2000_asize_0_merged_eyeglasses4000_results.png}} 
%  {}% 
% \hfill%
% \\  



% \jsubfig{\includegraphics[height=1.6cm]{latex/images/supplamentary/ratio_results/smiling_parameters_pairing_ratio_experiment/002661_real_A_smiling_paired_2000_2000_a2.png}} 
%  {}% 
% \hspace{3pt}
% \hfill%
% \jsubfig{\includegraphics[height=1.6cm]{latex/images/supplamentary/ratio_results/smiling_parameters_pairing_ratio_experiment/002661_fake_B_smiling_2000_with_2000_ratio_05_merged_eyeglasses4000_results.png}} 
%  {}% 
% \hfill%
% \jsubfig{\includegraphics[height=1.6cm]{latex/images/supplamentary/ratio_results/smiling_parameters_pairing_ratio_experiment/002661_fake_B_smiling_paired_2000_2000_a2_merged_eyeglasses4000_results.png}} 
%  {}% 
% \hfill%
% \jsubfig{\includegraphics[height=1.6cm]{latex/images/supplamentary/ratio_results/smiling_parameters_pairing_ratio_experiment/002661_fake_B_smiling_2000_with_2000_asize_200_merged_eyeglasses4000_results.png}} 
%  {}% 
% \hfill%
% \jsubfig{\includegraphics[height=1.6cm]{latex/images/supplamentary/ratio_results/smiling_parameters_pairing_ratio_experiment/002661_fake_B_smiling_2000_with_2000_asize_0_merged_eyeglasses4000_results.png}} 
%  {}% 
% \hfill%
% \\  



% \jsubfig{\includegraphics[height=1.6cm]{latex/images/supplamentary/ratio_results/smiling_parameters_pairing_ratio_experiment/002728_real_A_smiling_paired_2000_2000_a2.png}} 
%  {}% 
% \hspace{3pt}
% \hfill%
% \jsubfig{\includegraphics[height=1.6cm]{latex/images/supplamentary/ratio_results/smiling_parameters_pairing_ratio_experiment/002728_fake_B_smiling_2000_with_2000_ratio_05_merged_eyeglasses4000_results.png}} 
%  {}% 
% \hfill%
% \jsubfig{\includegraphics[height=1.6cm]{latex/images/supplamentary/ratio_results/smiling_parameters_pairing_ratio_experiment/002728_fake_B_smiling_paired_2000_2000_a2_merged_eyeglasses4000_results.png}} 
%  {}% 
% \hfill%
% \jsubfig{\includegraphics[height=1.6cm]{latex/images/supplamentary/ratio_results/smiling_parameters_pairing_ratio_experiment/002728_fake_B_smiling_2000_with_2000_asize_200_merged_eyeglasses4000_results.png}} 
%  {}% 
% \hfill%
% \jsubfig{\includegraphics[height=1.6cm]{latex/images/supplamentary/ratio_results/smiling_parameters_pairing_ratio_experiment/002728_fake_B_smiling_2000_with_2000_asize_0_merged_eyeglasses4000_results.png}} 
%  {}% 
% \hfill%
% \\  



% \jsubfig{\includegraphics[height=1.6cm]{latex/images/supplamentary/ratio_results/smiling_parameters_pairing_ratio_experiment/002745_real_A_smiling_paired_2000_2000_a2.png}} 
%  {Source}% 
% \hspace{3pt}
% \hfill%
% \jsubfig{\includegraphics[height=1.6cm]{latex/images/supplamentary/ratio_results/smiling_parameters_pairing_ratio_experiment/002745_fake_B_smiling_2000_with_2000_ratio_05_merged_eyeglasses4000_results.png}} 
%  {25\%}% 
% \hfill%
% \jsubfig{\includegraphics[height=1.6cm]{latex/images/supplamentary/ratio_results/smiling_parameters_pairing_ratio_experiment/002745_fake_B_smiling_paired_2000_2000_a2_merged_eyeglasses4000_results.png}} 
%  {50\%}% 
% \hfill%
% \jsubfig{\includegraphics[height=1.6cm]{latex/images/supplamentary/ratio_results/smiling_parameters_pairing_ratio_experiment/002745_fake_B_smiling_2000_with_2000_asize_200_merged_eyeglasses4000_results.png}} 
%  {90\%}% 
% \hfill%
% \jsubfig{\includegraphics[height=1.6cm]{latex/images/supplamentary/ratio_results/smiling_parameters_pairing_ratio_experiment/002745_fake_B_smiling_2000_with_2000_asize_0_merged_eyeglasses4000_results.png}} 
%  {100\%}% 
% \hfill%
% \vspace{3pt} 
 
%  \caption{Additional random pseudo-pair ratio analysis results for the  \emph{smile removal} task} 
%  \end{figure} 
