# Supplementary material for: Implicit Pairs for Boosting Unpaired Image-to-Image Translation
Source: arXiv:1904.06913 source file (2020-12-03)
Supplement: Supplementary file 3 [file smiling_training_regimes_old.tex]

% \begin{figure}
%   \centering% 
 
% \\  



% \jsubfig{\includegraphics[height=2.0cm]{latex/images/supplamentary/training_regimes/smiling_parameters_training_regimes_experiment/018822_real_A_smiling_paired_2000_2000_a2.png}} 
%  {}% 
% \hspace{3pt}
% \hfill%
% \jsubfig{\includegraphics[height=2.0cm]{latex/images/supplamentary/training_regimes/smiling_parameters_training_regimes_experiment/018822_fake_B_smiling_paired_2000_2000_a2_merged_eyeglasses4000_results.png}} 
%  {}% 
% \hfill%
% \jsubfig{\includegraphics[height=2.0cm]{latex/images/supplamentary/training_regimes/smiling_parameters_training_regimes_experiment/018822_fake_B_smiling_2000_with_2000_pix2pix_atob_merged_eyeglasses4000_results.png}} 
%  {}% 
% \hfill%
% \jsubfig{\includegraphics[height=2.0cm]{latex/images/supplamentary/training_regimes/smiling_parameters_training_regimes_experiment/018822_fake_B_smiling_2000_with_2000_implicitfirst_merged_eyeglasses4000_results.png}} 
%  {}% 
% \hfill%
% \\  



% \jsubfig{\includegraphics[height=2.0cm]{latex/images/supplamentary/training_regimes/smiling_parameters_training_regimes_experiment/018841_real_A_smiling_paired_2000_2000_a2.png}} 
%  {}% 
% \hspace{3pt}
% \hfill%
% \jsubfig{\includegraphics[height=2.0cm]{latex/images/supplamentary/training_regimes/smiling_parameters_training_regimes_experiment/018841_fake_B_smiling_paired_2000_2000_a2_merged_eyeglasses4000_results.png}} 
%  {}% 
% \hfill%
% \jsubfig{\includegraphics[height=2.0cm]{latex/images/supplamentary/training_regimes/smiling_parameters_training_regimes_experiment/018841_fake_B_smiling_2000_with_2000_pix2pix_atob_merged_eyeglasses4000_results.png}} 
%  {}% 
% \hfill%
% \jsubfig{\includegraphics[height=2.0cm]{latex/images/supplamentary/training_regimes/smiling_parameters_training_regimes_experiment/018841_fake_B_smiling_2000_with_2000_implicitfirst_merged_eyeglasses4000_results.png}} 
%  {}% 
% \hfill%
% \\  



% \jsubfig{\includegraphics[height=2.0cm]{latex/images/supplamentary/training_regimes/smiling_parameters_training_regimes_experiment/018875_real_A_smiling_paired_2000_2000_a2.png}} 
%  {}% 
% \hspace{3pt}
% \hfill%
% \jsubfig{\includegraphics[height=2.0cm]{latex/images/supplamentary/training_regimes/smiling_parameters_training_regimes_experiment/018875_fake_B_smiling_paired_2000_2000_a2_merged_eyeglasses4000_results.png}} 
%  {}% 
% \hfill%
% \jsubfig{\includegraphics[height=2.0cm]{latex/images/supplamentary/training_regimes/smiling_parameters_training_regimes_experiment/018875_fake_B_smiling_2000_with_2000_pix2pix_atob_merged_eyeglasses4000_results.png}} 
%  {}% 
% \hfill%
% \jsubfig{\includegraphics[height=2.0cm]{latex/images/supplamentary/training_regimes/smiling_parameters_training_regimes_experiment/018875_fake_B_smiling_2000_with_2000_implicitfirst_merged_eyeglasses4000_results.png}} 
%  {}% 
% \hfill%
% \\  



% \jsubfig{\includegraphics[height=2.0cm]{latex/images/supplamentary/training_regimes/smiling_parameters_training_regimes_experiment/018877_real_A_smiling_paired_2000_2000_a2.png}} 
%  {}% 
% \hspace{3pt}
% \hfill%
% \jsubfig{\includegraphics[height=2.0cm]{latex/images/supplamentary/training_regimes/smiling_parameters_training_regimes_experiment/018877_fake_B_smiling_paired_2000_2000_a2_merged_eyeglasses4000_results.png}} 
%  {}% 
% \hfill%
% \jsubfig{\includegraphics[height=2.0cm]{latex/images/supplamentary/training_regimes/smiling_parameters_training_regimes_experiment/018877_fake_B_smiling_2000_with_2000_pix2pix_atob_merged_eyeglasses4000_results.png}} 
%  {}% 
% \hfill%
% \jsubfig{\includegraphics[height=2.0cm]{latex/images/supplamentary/training_regimes/smiling_parameters_training_regimes_experiment/018877_fake_B_smiling_2000_with_2000_implicitfirst_merged_eyeglasses4000_results.png}} 
%  {}% 
% \hfill%
% \\  



% \jsubfig{\includegraphics[height=2.0cm]{latex/images/supplamentary/training_regimes/smiling_parameters_training_regimes_experiment/018881_real_A_smiling_paired_2000_2000_a2.png}} 
%  {}% 
% \hspace{3pt}
% \hfill%
% \jsubfig{\includegraphics[height=2.0cm]{latex/images/supplamentary/training_regimes/smiling_parameters_training_regimes_experiment/018881_fake_B_smiling_paired_2000_2000_a2_merged_eyeglasses4000_results.png}} 
%  {}% 
% \hfill%
% \jsubfig{\includegraphics[height=2.0cm]{latex/images/supplamentary/training_regimes/smiling_parameters_training_regimes_experiment/018881_fake_B_smiling_2000_with_2000_pix2pix_atob_merged_eyeglasses4000_results.png}} 
%  {}% 
% \hfill%
% \jsubfig{\includegraphics[height=2.0cm]{latex/images/supplamentary/training_regimes/smiling_parameters_training_regimes_experiment/018881_fake_B_smiling_2000_with_2000_implicitfirst_merged_eyeglasses4000_results.png}} 
%  {}% 
% \hfill%
% \\  



% \jsubfig{\includegraphics[height=2.0cm]{latex/images/supplamentary/training_regimes/smiling_parameters_training_regimes_experiment/022075_real_A_smiling_paired_2000_2000_a2.png}} 
%  {}% 
% \hspace{3pt}
% \hfill%
% \jsubfig{\includegraphics[height=2.0cm]{latex/images/supplamentary/training_regimes/smiling_parameters_training_regimes_experiment/022075_fake_B_smiling_paired_2000_2000_a2_merged_eyeglasses4000_results.png}} 
%  {}% 
% \hfill%
% \jsubfig{\includegraphics[height=2.0cm]{latex/images/supplamentary/training_regimes/smiling_parameters_training_regimes_experiment/022075_fake_B_smiling_2000_with_2000_pix2pix_atob_merged_eyeglasses4000_results.png}} 
%  {}% 
% \hfill%
% \jsubfig{\includegraphics[height=2.0cm]{latex/images/supplamentary/training_regimes/smiling_parameters_training_regimes_experiment/022075_fake_B_smiling_2000_with_2000_implicitfirst_merged_eyeglasses4000_results.png}} 
%  {}% 
% \hfill%
% \\  



% \jsubfig{\includegraphics[height=2.0cm]{latex/images/supplamentary/training_regimes/smiling_parameters_training_regimes_experiment/022076_real_A_smiling_paired_2000_2000_a2.png}} 
%  {}% 
% \hspace{3pt}
% \hfill%
% \jsubfig{\includegraphics[height=2.0cm]{latex/images/supplamentary/training_regimes/smiling_parameters_training_regimes_experiment/022076_fake_B_smiling_paired_2000_2000_a2_merged_eyeglasses4000_results.png}} 
%  {}% 
% \hfill%
% \jsubfig{\includegraphics[height=2.0cm]{latex/images/supplamentary/training_regimes/smiling_parameters_training_regimes_experiment/022076_fake_B_smiling_2000_with_2000_pix2pix_atob_merged_eyeglasses4000_results.png}} 
%  {}% 
% \hfill%
% \jsubfig{\includegraphics[height=2.0cm]{latex/images/supplamentary/training_regimes/smiling_parameters_training_regimes_experiment/022076_fake_B_smiling_2000_with_2000_implicitfirst_merged_eyeglasses4000_results.png}} 
%  {}% 
% \hfill%
% \\  



% \jsubfig{\includegraphics[height=2.0cm]{latex/images/supplamentary/training_regimes/smiling_parameters_training_regimes_experiment/022089_real_A_smiling_paired_2000_2000_a2.png}} 
%  {}% 
% \hspace{3pt}
% \hfill%
% \jsubfig{\includegraphics[height=2.0cm]{latex/images/supplamentary/training_regimes/smiling_parameters_training_regimes_experiment/022089_fake_B_smiling_paired_2000_2000_a2_merged_eyeglasses4000_results.png}} 
%  {}% 
% \hfill%
% \jsubfig{\includegraphics[height=2.0cm]{latex/images/supplamentary/training_regimes/smiling_parameters_training_regimes_experiment/022089_fake_B_smiling_2000_with_2000_pix2pix_atob_merged_eyeglasses4000_results.png}} 
%  {}% 
% \hfill%
% \jsubfig{\includegraphics[height=2.0cm]{latex/images/supplamentary/training_regimes/smiling_parameters_training_regimes_experiment/022089_fake_B_smiling_2000_with_2000_implicitfirst_merged_eyeglasses4000_results.png}} 
%  {}% 
% \hfill%
% \\  



% \jsubfig{\includegraphics[height=2.0cm]{latex/images/supplamentary/training_regimes/smiling_parameters_training_regimes_experiment/022118_real_A_smiling_paired_2000_2000_a2.png}} 
%  {}% 
% \hspace{3pt}
% \hfill%
% \jsubfig{\includegraphics[height=2.0cm]{latex/images/supplamentary/training_regimes/smiling_parameters_training_regimes_experiment/022118_fake_B_smiling_paired_2000_2000_a2_merged_eyeglasses4000_results.png}} 
%  {}% 
% \hfill%
% \jsubfig{\includegraphics[height=2.0cm]{latex/images/supplamentary/training_regimes/smiling_parameters_training_regimes_experiment/022118_fake_B_smiling_2000_with_2000_pix2pix_atob_merged_eyeglasses4000_results.png}} 
%  {}% 
% \hfill%
% \jsubfig{\includegraphics[height=2.0cm]{latex/images/supplamentary/training_regimes/smiling_parameters_training_regimes_experiment/022118_fake_B_smiling_2000_with_2000_implicitfirst_merged_eyeglasses4000_results.png}} 
%  {}% 
% \hfill%
% \\  



% \jsubfig{\includegraphics[height=2.0cm]{latex/images/supplamentary/training_regimes/smiling_parameters_training_regimes_experiment/022131_real_A_smiling_paired_2000_2000_a2.png}} 
%  {Source}% 
% \hspace{3pt}
% \hfill%
% \jsubfig{\includegraphics[height=2.0cm]{latex/images/supplamentary/training_regimes/smiling_parameters_training_regimes_experiment/022131_fake_B_smiling_paired_2000_2000_a2_merged_eyeglasses4000_results.png}} 
%  {Implicit}% 
% \hfill%
% \jsubfig{\includegraphics[height=2.0cm]{latex/images/supplamentary/training_regimes/smiling_parameters_training_regimes_experiment/022131_fake_B_smiling_2000_with_2000_pix2pix_atob_merged_eyeglasses4000_results.png}} 
%  {Explicit}% 
% \hfill%
% \jsubfig{\includegraphics[height=2.0cm]{latex/images/supplamentary/training_regimes/smiling_parameters_training_regimes_experiment/022131_fake_B_smiling_2000_with_2000_implicitfirst_merged_eyeglasses4000_results.png}} 
%  {Semi-explicit}% 
% \hfill%
% \\  



% % \jsubfig{\includegraphics[height=2.0cm]{latex/images/supplamentary/training_regimes/smiling_parameters_training_regimes_experiment/010863_real_A_smiling_paired_2000_2000_a2.png}} 
% %  {}% 
% % \hspace{3pt}
% % \hfill%
% % \jsubfig{\includegraphics[height=2.0cm]{latex/images/supplamentary/training_regimes/smiling_parameters_training_regimes_experiment/010863_fake_B_smiling_paired_2000_2000_a2_merged_eyeglasses4000_results.png}} 
% %  {}% 
% % \hfill%
% % \jsubfig{\includegraphics[height=2.0cm]{latex/images/supplamentary/training_regimes/smiling_parameters_training_regimes_experiment/010863_fake_B_smiling_2000_with_2000_pix2pix_atob_merged_eyeglasses4000_results.png}} 
% %  {}% 
% % \hfill%
% % \jsubfig{\includegraphics[height=2.0cm]{latex/images/supplamentary/training_regimes/smiling_parameters_training_regimes_experiment/010863_fake_B_smiling_2000_with_2000_implicitfirst_merged_eyeglasses4000_results.png}} 
% %  {}% 
% % \hfill%
% % \\  



% % \jsubfig{\includegraphics[height=2.0cm]{latex/images/supplamentary/training_regimes/smiling_parameters_training_regimes_experiment/010887_real_A_smiling_paired_2000_2000_a2.png}} 
% %  {}% 
% % \hspace{3pt}
% % \hfill%
% % \jsubfig{\includegraphics[height=2.0cm]{latex/images/supplamentary/training_regimes/smiling_parameters_training_regimes_experiment/010887_fake_B_smiling_paired_2000_2000_a2_merged_eyeglasses4000_results.png}} 
% %  {}% 
% % \hfill%
% % \jsubfig{\includegraphics[height=2.0cm]{latex/images/supplamentary/training_regimes/smiling_parameters_training_regimes_experiment/010887_fake_B_smiling_2000_with_2000_pix2pix_atob_merged_eyeglasses4000_results.png}} 
% %  {}% 
% % \hfill%
% % \jsubfig{\includegraphics[height=2.0cm]{latex/images/supplamentary/training_regimes/smiling_parameters_training_regimes_experiment/010887_fake_B_smiling_2000_with_2000_implicitfirst_merged_eyeglasses4000_results.png}} 
% %  {}% 
% % \hfill%
% % \\  



% % \jsubfig{\includegraphics[height=2.0cm]{latex/images/supplamentary/training_regimes/smiling_parameters_training_regimes_experiment/010909_real_A_smiling_paired_2000_2000_a2.png}} 
% %  {}% 
% % \hspace{3pt}
% % \hfill%
% % \jsubfig{\includegraphics[height=2.0cm]{latex/images/supplamentary/training_regimes/smiling_parameters_training_regimes_experiment/010909_fake_B_smiling_paired_2000_2000_a2_merged_eyeglasses4000_results.png}} 
% %  {}% 
% % \hfill%
% % \jsubfig{\includegraphics[height=2.0cm]{latex/images/supplamentary/training_regimes/smiling_parameters_training_regimes_experiment/010909_fake_B_smiling_2000_with_2000_pix2pix_atob_merged_eyeglasses4000_results.png}} 
% %  {}% 
% % \hfill%
% % \jsubfig{\includegraphics[height=2.0cm]{latex/images/supplamentary/training_regimes/smiling_parameters_training_regimes_experiment/010909_fake_B_smiling_2000_with_2000_implicitfirst_merged_eyeglasses4000_results.png}} 
% %  {}% 
% % \hfill%
% % \\  



% % \jsubfig{\includegraphics[height=2.0cm]{latex/images/supplamentary/training_regimes/smiling_parameters_training_regimes_experiment/010934_real_A_smiling_paired_2000_2000_a2.png}} 
% %  {}% 
% % \hspace{3pt}
% % \hfill%
% % \jsubfig{\includegraphics[height=2.0cm]{latex/images/supplamentary/training_regimes/smiling_parameters_training_regimes_experiment/010934_fake_B_smiling_paired_2000_2000_a2_merged_eyeglasses4000_results.png}} 
% %  {}% 
% % \hfill%
% % \jsubfig{\includegraphics[height=2.0cm]{latex/images/supplamentary/training_regimes/smiling_parameters_training_regimes_experiment/010934_fake_B_smiling_2000_with_2000_pix2pix_atob_merged_eyeglasses4000_results.png}} 
% %  {}% 
% % \hfill%
% % \jsubfig{\includegraphics[height=2.0cm]{latex/images/supplamentary/training_regimes/smiling_parameters_training_regimes_experiment/010934_fake_B_smiling_2000_with_2000_implicitfirst_merged_eyeglasses4000_results.png}} 
% %  {}% 
% % \hfill%
% % \\  



% % \jsubfig{\includegraphics[height=2.0cm]{latex/images/supplamentary/training_regimes/smiling_parameters_training_regimes_experiment/010939_real_A_smiling_paired_2000_2000_a2.png}} 
% %  {}% 
% % \hspace{3pt}
% % \hfill%
% % \jsubfig{\includegraphics[height=2.0cm]{latex/images/supplamentary/training_regimes/smiling_parameters_training_regimes_experiment/010939_fake_B_smiling_paired_2000_2000_a2_merged_eyeglasses4000_results.png}} 
% %  {}% 
% % \hfill%
% % \jsubfig{\includegraphics[height=2.0cm]{latex/images/supplamentary/training_regimes/smiling_parameters_training_regimes_experiment/010939_fake_B_smiling_2000_with_2000_pix2pix_atob_merged_eyeglasses4000_results.png}} 
% %  {}% 
% % \hfill%
% % \jsubfig{\includegraphics[height=2.0cm]{latex/images/supplamentary/training_regimes/smiling_parameters_training_regimes_experiment/010939_fake_B_smiling_2000_with_2000_implicitfirst_merged_eyeglasses4000_results.png}} 
% %  {}% 
% % \hfill%
% \vspace{3pt} 
 
%  \caption{Additional random \emph{Smile removal} results with pseudo-pairs in different settings.} 
%  % \label{} 
%  \end{figure} 
